# Supplementary material for: Spatio-Temporal Action Detection Under Large Motion
Source: arXiv:2209.02250 source file (2022-10-25)
Supplement: Supplementary file 7 [file TAB_AVA_supp.tex]

\begin{table}[t!]
    %\vskip -3mm
    \centering
    % \captionsetup{font=footnotesize}
    \footnotesize
    \setlength{\tabcolsep}{8pt}
    
    \caption{%Results of different method under different action motion speed, .
    \motionap{} ablation on AVA dataset.
    }
    \vspace{-1.0em}
    % \vskip 2mm
    %\resizebox{1.00\linewidth}{!}{
    % \begin{tabular}{lcccccccc}
    \begin{tabular}{lllll}
    \toprule
     & \fmap{} & \multicolumn{3}{c}{\motionap{}} \\
    Method & @0.5   &  Large & Medium & Small \\
    \midrule
    Baseline & - & - & - & -   \\
    Baseline + track${}^{*}$ & -\small{(+-.-)} & --\small{(+-.-)} & -\small{(+-.-)} & --\small{(+-.-)}  \\ 
    % \taad+\maxpool & 53.9\small{(+4.3)}  & 70.2\small{(+7.0)} & 83.4\small{(\textbf{+5.7})} & 86.1\small{(+3.9)}  \\
    \taad+\aspp & --\small{(+-.-)}  & --\small{(\textbf{+-.-})}  & --\small{(\textbf{+-.-})} & --\small{(+-.-)}  \\
    % \taad+\tcn & 55.3\small{(\textbf{+5.7})} & 70.4\small{(+7.2)} & 83.3\small{(+5.6)} & 87.3\small{(\textbf{+4.9})}\\
    % % \midrule
    \bottomrule
    %\multicolumn{5}{l}{${}^{*}$ track boxes scored using baseline, tracks act as false-positive filtering module.}
    \end{tabular}
    %}
    \label{tab:motion_ava_ap} 
    \vspace{-2.0em}
\end{table}
